# Supplementary material for: Nonlocal energy density functionals for low-energy nuclear structure
Source: arXiv:1402.1556 source file (2014-02-07)
Supplement: Supplementary file 5 [file Suppl_T_Section_3_N2LO.tex]

%auto-ignore
%% AMS-LaTeX Created by Wolfram Mathematica 7.0 : www.wolfram.com

\documentclass{article}
\usepackage{amsmath, amssymb, graphics}

\newcommand{\mathsym}[1]{{}}
\newcommand{\unicode}{{}}

\begin{document}

\noindent\(C_{00,2000,0}^{00,2000,0,\text{Loc}}\longrightarrow \frac{5 C_{00,00}^{40,0}}{48}+\frac{5 C_{00,00}^{40,1}}{96}+\frac{5 C_{11,00}^{31,0}}{48}+\frac{5
C_{11,00}^{31,1}}{96}+\frac{5 C_{20,00}^{20,0}}{48}+\frac{5 C_{20,00}^{20,1}}{96}+\frac{\sqrt{5} C_{22,00}^{22,0}}{24}+\frac{\sqrt{5} C_{22,00}^{22,1}}{48}\)

\noindent\(C_{00,2000,0}^{00,2000,0,\text{NonLoc}}\longrightarrow -\frac{5 C_{00,00}^{40,0}}{192}-\frac{5 C_{00,00}^{40,1}}{96}+\frac{5 C_{00,20}^{40,0}}{64
\sqrt{3}}+\frac{5 C_{00,20}^{40,1}}{32 \sqrt{3}}+\frac{5 C_{11,00}^{31,0}}{192}+\frac{5 C_{11,00}^{31,1}}{96}-\frac{5 C_{11,20}^{31,0}}{64 \sqrt{3}}-\frac{5
C_{11,20}^{31,1}}{32 \sqrt{3}}-\frac{5 C_{20,00}^{20,0}}{192}-\frac{5 C_{20,00}^{20,1}}{96}+\frac{5 C_{20,20}^{20,0}}{64 \sqrt{3}}+\frac{5 C_{20,20}^{20,1}}{32
\sqrt{3}}-\frac{\sqrt{5} C_{22,00}^{22,0}}{96}-\frac{\sqrt{5} C_{22,00}^{22,1}}{48}+\frac{1}{32} \sqrt{\frac{5}{3}} C_{22,20}^{22,0}+\frac{1}{16}
\sqrt{\frac{5}{3}} C_{22,20}^{22,1}\)

\noindent\(C_{00,4000,0}^{00,0000,0,\text{Loc}}\longrightarrow \frac{C_{00,00}^{40,0}}{16}+\frac{C_{00,00}^{40,1}}{32}+\frac{C_{11,00}^{31,0}}{16}+\frac{C_{11,00}^{31,1}}{32}+\frac{C_{20,00}^{20,0}}{16}+\frac{C_{20,00}^{20,1}}{32}+\frac{C_{22,00}^{22,0}}{8
\sqrt{5}}+\frac{C_{22,00}^{22,1}}{16 \sqrt{5}}\)

\noindent\(C_{00,4000,0}^{00,0000,0,\text{NonLoc}}\longrightarrow -\frac{C_{00,00}^{40,0}}{64}-\frac{C_{00,00}^{40,1}}{32}+\frac{\sqrt{3} C_{00,20}^{40,0}}{64}+\frac{\sqrt{3}
C_{00,20}^{40,1}}{32}+\frac{C_{11,00}^{31,0}}{64}+\frac{C_{11,00}^{31,1}}{32}-\frac{\sqrt{3} C_{11,20}^{31,0}}{64}-\frac{\sqrt{3} C_{11,20}^{31,1}}{32}-\frac{C_{20,00}^{20,0}}{64}-\frac{C_{20,00}^{20,1}}{32}+\frac{\sqrt{3}
C_{20,20}^{20,0}}{64}+\frac{\sqrt{3} C_{20,20}^{20,1}}{32}-\frac{C_{22,00}^{22,0}}{32 \sqrt{5}}-\frac{C_{22,00}^{22,1}}{16 \sqrt{5}}+\frac{1}{32}
\sqrt{\frac{3}{5}} C_{22,20}^{22,0}+\frac{1}{16} \sqrt{\frac{3}{5}} C_{22,20}^{22,1}\)

\noindent\(C_{20,0000,0}^{00,2000,0,\text{NonLoc}}\longrightarrow \frac{5 C_{00,00}^{40,0}}{384}+\frac{5 C_{00,00}^{40,1}}{192}-\frac{5 C_{00,20}^{40,0}}{128
\sqrt{3}}-\frac{5 C_{00,20}^{40,1}}{64 \sqrt{3}}+\frac{C_{20,00}^{20,0}}{384}+\frac{C_{20,00}^{20,1}}{192}-\frac{C_{20,20}^{20,0}}{128 \sqrt{3}}-\frac{C_{20,20}^{20,1}}{64
\sqrt{3}}-\frac{\sqrt{5} C_{22,00}^{22,0}}{192}-\frac{\sqrt{5} C_{22,00}^{22,1}}{96}+\frac{1}{64} \sqrt{\frac{5}{3}} C_{22,20}^{22,0}+\frac{1}{32}
\sqrt{\frac{5}{3}} C_{22,20}^{22,1}\)

\noindent\(C_{20,0000,0}^{20,0000,0,\text{NonLoc}}\longrightarrow -\frac{5 C_{00,00}^{40,0}}{3072}-\frac{5 C_{00,00}^{40,1}}{1536}+\frac{5 C_{00,20}^{40,0}}{1024
\sqrt{3}}+\frac{5 C_{00,20}^{40,1}}{512 \sqrt{3}}-\frac{5 C_{11,00}^{31,0}}{3072}-\frac{5 C_{11,00}^{31,1}}{1536}+\frac{5 C_{11,20}^{31,0}}{1024
\sqrt{3}}+\frac{5 C_{11,20}^{31,1}}{512 \sqrt{3}}-\frac{5 C_{20,00}^{20,0}}{3072}-\frac{5 C_{20,00}^{20,1}}{1536}+\frac{5 C_{20,20}^{20,0}}{1024
\sqrt{3}}+\frac{5 C_{20,20}^{20,1}}{512 \sqrt{3}}-\frac{\sqrt{5} C_{22,00}^{22,0}}{1536}-\frac{\sqrt{5} C_{22,00}^{22,1}}{768}+\frac{1}{512} \sqrt{\frac{5}{3}}
C_{22,20}^{22,0}+\frac{1}{256} \sqrt{\frac{5}{3}} C_{22,20}^{22,1}\)

\noindent\(C_{20,2000,0}^{00,0000,0,\text{NonLoc}}\longrightarrow \frac{5 C_{00,00}^{40,0}}{384}+\frac{5 C_{00,00}^{40,1}}{192}-\frac{5 C_{00,20}^{40,0}}{128
\sqrt{3}}-\frac{5 C_{00,20}^{40,1}}{64 \sqrt{3}}+\frac{C_{20,00}^{20,0}}{384}+\frac{C_{20,00}^{20,1}}{192}-\frac{C_{20,20}^{20,0}}{128 \sqrt{3}}-\frac{C_{20,20}^{20,1}}{64
\sqrt{3}}-\frac{\sqrt{5} C_{22,00}^{22,0}}{192}-\frac{\sqrt{5} C_{22,00}^{22,1}}{96}+\frac{1}{64} \sqrt{\frac{5}{3}} C_{22,20}^{22,0}+\frac{1}{32}
\sqrt{\frac{5}{3}} C_{22,20}^{22,1}\)

\noindent\(C_{40,0000,0}^{00,0000,0,\text{NonLoc}}\longrightarrow -\frac{C_{00,00}^{40,0}}{1024}-\frac{C_{00,00}^{40,1}}{512}+\frac{\sqrt{3} C_{00,20}^{40,0}}{1024}+\frac{\sqrt{3}
C_{00,20}^{40,1}}{512}-\frac{C_{11,00}^{31,0}}{1024}-\frac{C_{11,00}^{31,1}}{512}+\frac{\sqrt{3} C_{11,20}^{31,0}}{1024}+\frac{\sqrt{3} C_{11,20}^{31,1}}{512}-\frac{C_{20,00}^{20,0}}{1024}-\frac{C_{20,00}^{20,1}}{512}+\frac{\sqrt{3}
C_{20,20}^{20,0}}{1024}+\frac{\sqrt{3} C_{20,20}^{20,1}}{512}-\frac{C_{22,00}^{22,0}}{512 \sqrt{5}}-\frac{C_{22,00}^{22,1}}{256 \sqrt{5}}+\frac{1}{512}
\sqrt{\frac{3}{5}} C_{22,20}^{22,0}+\frac{1}{256} \sqrt{\frac{3}{5}} C_{22,20}^{22,1}\)

\end{document}
