# Supplementary material for: Nonlocal energy density functionals for low-energy nuclear structure
Source: arXiv:1402.1556 source file (2014-02-07)
Supplement: Supplementary file 6 [file Suppl_T_Section_3_N3LO.tex]

%auto-ignore
%% AMS-LaTeX Created by Wolfram Mathematica 7.0 : www.wolfram.com

\documentclass{article}
\usepackage{amsmath, amssymb, graphics}

\newcommand{\mathsym}[1]{{}}
\newcommand{\unicode}{{}}

\begin{document}

\noindent\(C_{00,4000,0}^{00,2000,0,\text{Loc}}\longrightarrow \frac{7 C_{00,00}^{60,0}}{64}+\frac{7 C_{00,00}^{60,1}}{128}+\frac{7 C_{11,00}^{51,0}}{64}+\frac{7
C_{11,00}^{51,1}}{128}+\frac{7 C_{20,00}^{40,0}}{64}+\frac{7 C_{20,00}^{40,1}}{128}+\frac{7 C_{22,00}^{42,0}}{32 \sqrt{5}}+\frac{7 C_{22,00}^{42,1}}{64
\sqrt{5}}+\frac{7 C_{31,00}^{31,0}}{64}+\frac{7 C_{31,00}^{31,1}}{128}+\frac{3 \sqrt{21} C_{33,00}^{33,0}}{160}+\frac{3 \sqrt{21} C_{33,00}^{33,1}}{320}\)

\noindent\(C_{00,4000,0}^{00,2000,0,\text{NonLoc}}\longrightarrow -\frac{7 C_{00,00}^{60,0}}{256}-\frac{7 C_{00,00}^{60,1}}{128}+\frac{7 \sqrt{3}
C_{00,20}^{60,0}}{256}+\frac{7 \sqrt{3} C_{00,20}^{60,1}}{128}+\frac{7 C_{11,00}^{51,0}}{256}+\frac{7 C_{11,00}^{51,1}}{128}-\frac{7 \sqrt{3} C_{11,20}^{31,0}}{512}-\frac{7
\sqrt{3} C_{11,20}^{31,1}}{256}-\frac{7 C_{20,00}^{40,0}}{256}-\frac{7 C_{20,00}^{40,1}}{128}+\frac{7 \sqrt{3} C_{20,20}^{40,0}}{256}+\frac{7 \sqrt{3}
C_{20,20}^{40,1}}{128}-\frac{7 C_{22,00}^{42,0}}{128 \sqrt{5}}-\frac{7 C_{22,00}^{42,1}}{64 \sqrt{5}}+\frac{7}{128} \sqrt{\frac{3}{5}} C_{22,20}^{42,0}+\frac{7}{64}
\sqrt{\frac{3}{5}} C_{22,20}^{42,1}+\frac{7 C_{31,00}^{31,0}}{256}+\frac{7 C_{31,00}^{31,1}}{128}-\frac{7 \sqrt{3} C_{31,20}^{31,0}}{256}-\frac{7
\sqrt{3} C_{31,20}^{31,1}}{128}+\frac{3 \sqrt{21} C_{33,00}^{33,0}}{640}+\frac{3 \sqrt{21} C_{33,00}^{33,1}}{320}-\frac{9 \sqrt{7} C_{33,20}^{33,0}}{640}-\frac{9
\sqrt{7} C_{33,20}^{33,1}}{320}\)

\noindent\(C_{00,6000,0}^{00,0000,0,\text{Loc}}\longrightarrow \frac{C_{00,00}^{60,0}}{64}+\frac{C_{00,00}^{60,1}}{128}+\frac{C_{11,00}^{51,0}}{64}+\frac{C_{11,00}^{51,1}}{128}+\frac{C_{20,00}^{40,0}}{64}+\frac{C_{20,00}^{40,1}}{128}+\frac{C_{22,00}^{42,0}}{32
\sqrt{5}}+\frac{C_{22,00}^{42,1}}{64 \sqrt{5}}+\frac{C_{31,00}^{31,0}}{64}+\frac{C_{31,00}^{31,1}}{128}+\frac{3}{160} \sqrt{\frac{3}{7}} C_{33,00}^{33,0}+\frac{3}{320}
\sqrt{\frac{3}{7}} C_{33,00}^{33,1}\)

\noindent\(C_{00,6000,0}^{00,0000,0,\text{NonLoc}}\longrightarrow -\frac{C_{00,00}^{60,0}}{256}-\frac{C_{00,00}^{60,1}}{128}+\frac{\sqrt{3} C_{00,20}^{60,0}}{256}+\frac{\sqrt{3}
C_{00,20}^{60,1}}{128}+\frac{C_{11,00}^{51,0}}{256}+\frac{C_{11,00}^{51,1}}{128}-\frac{\sqrt{3} C_{11,20}^{31,0}}{256}-\frac{\sqrt{3} C_{11,20}^{31,1}}{128}-\frac{C_{20,00}^{40,0}}{256}-\frac{C_{20,00}^{40,1}}{128}+\frac{\sqrt{3}
C_{20,20}^{40,0}}{256}+\frac{\sqrt{3} C_{20,20}^{40,1}}{128}-\frac{C_{22,00}^{42,0}}{128 \sqrt{5}}-\frac{C_{22,00}^{42,1}}{64 \sqrt{5}}+\frac{1}{128}
\sqrt{\frac{3}{5}} C_{22,20}^{42,0}+\frac{1}{64} \sqrt{\frac{3}{5}} C_{22,20}^{42,1}+\frac{C_{31,00}^{31,0}}{256}+\frac{C_{31,00}^{31,1}}{128}-\frac{\sqrt{3}
C_{31,20}^{31,0}}{256}-\frac{\sqrt{3} C_{31,20}^{31,1}}{128}+\frac{3}{640} \sqrt{\frac{3}{7}} C_{33,00}^{33,0}+\frac{3}{320} \sqrt{\frac{3}{7}} C_{33,00}^{33,1}-\frac{9
C_{33,20}^{33,0}}{640 \sqrt{7}}-\frac{9 C_{33,20}^{33,1}}{320 \sqrt{7}}\)

\noindent\(C_{20,0000,0}^{00,4000,0,\text{NonLoc}}\longrightarrow \frac{7 C_{00,00}^{60,0}}{1024}+\frac{7 C_{00,00}^{60,1}}{512}-\frac{7 \sqrt{3}
C_{00,20}^{60,0}}{1024}-\frac{7 \sqrt{3} C_{00,20}^{60,1}}{512}-\frac{7 C_{11,00}^{51,0}}{3072}-\frac{7 C_{11,00}^{51,1}}{1536}+\frac{7 C_{11,20}^{31,0}}{2048
\sqrt{3}}+\frac{7 C_{11,20}^{31,1}}{1024 \sqrt{3}}+\frac{5 C_{20,00}^{40,0}}{3072}+\frac{5 C_{20,00}^{40,1}}{1536}-\frac{5 C_{20,20}^{40,0}}{1024
\sqrt{3}}-\frac{5 C_{20,20}^{40,1}}{512 \sqrt{3}}-\frac{7 C_{22,00}^{42,0}}{1536 \sqrt{5}}-\frac{7 C_{22,00}^{42,1}}{768 \sqrt{5}}+\frac{7 C_{22,20}^{42,0}}{512
\sqrt{15}}+\frac{7 C_{22,20}^{42,1}}{256 \sqrt{15}}+\frac{C_{31,00}^{31,0}}{3072}+\frac{C_{31,00}^{31,1}}{1536}-\frac{C_{31,20}^{31,0}}{1024 \sqrt{3}}-\frac{C_{31,20}^{31,1}}{512
\sqrt{3}}+\frac{3 \sqrt{21} C_{33,00}^{33,0}}{2560}+\frac{3 \sqrt{21} C_{33,00}^{33,1}}{1280}-\frac{9 \sqrt{7} C_{33,20}^{33,0}}{2560}-\frac{9 \sqrt{7}
C_{33,20}^{33,1}}{1280}\)

\noindent\(C_{20,2000,0}^{00,2000,0,\text{NonLoc}}\longrightarrow \frac{35 C_{00,00}^{60,0}}{1536}+\frac{35 C_{00,00}^{60,1}}{768}-\frac{35 C_{00,20}^{60,0}}{512
\sqrt{3}}-\frac{35 C_{00,20}^{60,1}}{256 \sqrt{3}}-\frac{35 C_{11,00}^{51,0}}{4608}-\frac{35 C_{11,00}^{51,1}}{2304}+\frac{35 C_{11,20}^{31,0}}{1536
\sqrt{3}}+\frac{35 C_{11,20}^{31,1}}{768 \sqrt{3}}+\frac{25 C_{20,00}^{40,0}}{4608}+\frac{25 C_{20,00}^{40,1}}{2304}-\frac{25 C_{20,20}^{40,0}}{1536
\sqrt{3}}-\frac{25 C_{20,20}^{40,1}}{768 \sqrt{3}}-\frac{7 \sqrt{5} C_{22,00}^{42,0}}{2304}-\frac{7 \sqrt{5} C_{22,00}^{42,1}}{1152}+\frac{7}{768}
\sqrt{\frac{5}{3}} C_{22,20}^{42,0}+\frac{7}{384} \sqrt{\frac{5}{3}} C_{22,20}^{42,1}+\frac{5 C_{31,00}^{31,0}}{4608}+\frac{5 C_{31,00}^{31,1}}{2304}-\frac{5
C_{31,20}^{31,0}}{1536 \sqrt{3}}-\frac{5 C_{31,20}^{31,1}}{768 \sqrt{3}}+\frac{\sqrt{21} C_{33,00}^{33,0}}{256}+\frac{\sqrt{21} C_{33,00}^{33,1}}{128}-\frac{3
\sqrt{7} C_{33,20}^{33,0}}{256}-\frac{3 \sqrt{7} C_{33,20}^{33,1}}{128}\)

\noindent\(C_{20,2000,0}^{20,0000,0,\text{NonLoc}}\longrightarrow -\frac{35 C_{00,00}^{60,0}}{6144}-\frac{35 C_{00,00}^{60,1}}{3072}+\frac{35 C_{00,20}^{60,0}}{2048
\sqrt{3}}+\frac{35 C_{00,20}^{60,1}}{1024 \sqrt{3}}-\frac{35 C_{11,00}^{51,0}}{18432}-\frac{35 C_{11,00}^{51,1}}{9216}+\frac{35 C_{11,20}^{31,0}}{6144
\sqrt{3}}+\frac{35 C_{11,20}^{31,1}}{3072 \sqrt{3}}-\frac{25 C_{20,00}^{40,0}}{18432}-\frac{25 C_{20,00}^{40,1}}{9216}+\frac{25 C_{20,20}^{40,0}}{6144
\sqrt{3}}+\frac{25 C_{20,20}^{40,1}}{3072 \sqrt{3}}+\frac{7 \sqrt{5} C_{22,00}^{42,0}}{9216}+\frac{7 \sqrt{5} C_{22,00}^{42,1}}{4608}-\frac{7 \sqrt{\frac{5}{3}}
C_{22,20}^{42,0}}{3072}-\frac{7 \sqrt{\frac{5}{3}} C_{22,20}^{42,1}}{1536}+\frac{5 C_{31,00}^{31,0}}{18432}+\frac{5 C_{31,00}^{31,1}}{9216}-\frac{5
C_{31,20}^{31,0}}{6144 \sqrt{3}}-\frac{5 C_{31,20}^{31,1}}{3072 \sqrt{3}}+\frac{\sqrt{21} C_{33,00}^{33,0}}{1024}+\frac{\sqrt{21} C_{33,00}^{33,1}}{512}-\frac{3
\sqrt{7} C_{33,20}^{33,0}}{1024}-\frac{3 \sqrt{7} C_{33,20}^{33,1}}{512}\)

\noindent\(C_{20,4000,0}^{00,0000,0,\text{NonLoc}}\longrightarrow \frac{7 C_{00,00}^{60,0}}{1024}+\frac{7 C_{00,00}^{60,1}}{512}-\frac{7 \sqrt{3}
C_{00,20}^{60,0}}{1024}-\frac{7 \sqrt{3} C_{00,20}^{60,1}}{512}-\frac{7 C_{11,00}^{51,0}}{3072}-\frac{7 C_{11,00}^{51,1}}{1536}+\frac{7 C_{11,20}^{31,0}}{1024
\sqrt{3}}+\frac{7 C_{11,20}^{31,1}}{512 \sqrt{3}}+\frac{5 C_{20,00}^{40,0}}{3072}+\frac{5 C_{20,00}^{40,1}}{1536}-\frac{5 C_{20,20}^{40,0}}{1024
\sqrt{3}}-\frac{5 C_{20,20}^{40,1}}{512 \sqrt{3}}-\frac{7 C_{22,00}^{42,0}}{1536 \sqrt{5}}-\frac{7 C_{22,00}^{42,1}}{768 \sqrt{5}}+\frac{7 C_{22,20}^{42,0}}{512
\sqrt{15}}+\frac{7 C_{22,20}^{42,1}}{256 \sqrt{15}}+\frac{C_{31,00}^{31,0}}{3072}+\frac{C_{31,00}^{31,1}}{1536}-\frac{C_{31,20}^{31,0}}{1024 \sqrt{3}}-\frac{C_{31,20}^{31,1}}{512
\sqrt{3}}+\frac{3 \sqrt{21} C_{33,00}^{33,0}}{2560}+\frac{3 \sqrt{21} C_{33,00}^{33,1}}{1280}-\frac{9 \sqrt{7} C_{33,20}^{33,0}}{2560}-\frac{9 \sqrt{7}
C_{33,20}^{33,1}}{1280}\)

\noindent\(C_{40,0000,0}^{00,2000,0,\text{NonLoc}}\longrightarrow -\frac{7 C_{00,00}^{60,0}}{4096}-\frac{7 C_{00,00}^{60,1}}{2048}+\frac{7 \sqrt{3}
C_{00,20}^{60,0}}{4096}+\frac{7 \sqrt{3} C_{00,20}^{60,1}}{2048}-\frac{7 C_{11,00}^{51,0}}{12288}-\frac{7 C_{11,00}^{51,1}}{6144}+\frac{7 C_{11,20}^{31,0}}{8192
\sqrt{3}}+\frac{7 C_{11,20}^{31,1}}{4096 \sqrt{3}}-\frac{5 C_{20,00}^{40,0}}{12288}-\frac{5 C_{20,00}^{40,1}}{6144}+\frac{5 C_{20,20}^{40,0}}{4096
\sqrt{3}}+\frac{5 C_{20,20}^{40,1}}{2048 \sqrt{3}}+\frac{7 C_{22,00}^{42,0}}{6144 \sqrt{5}}+\frac{7 C_{22,00}^{42,1}}{3072 \sqrt{5}}-\frac{7 C_{22,20}^{42,0}}{2048
\sqrt{15}}-\frac{7 C_{22,20}^{42,1}}{1024 \sqrt{15}}+\frac{C_{31,00}^{31,0}}{12288}+\frac{C_{31,00}^{31,1}}{6144}-\frac{C_{31,20}^{31,0}}{4096 \sqrt{3}}-\frac{C_{31,20}^{31,1}}{2048
\sqrt{3}}+\frac{3 \sqrt{21} C_{33,00}^{33,0}}{10240}+\frac{3 \sqrt{21} C_{33,00}^{33,1}}{5120}-\frac{9 \sqrt{7} C_{33,20}^{33,0}}{10240}-\frac{9
\sqrt{7} C_{33,20}^{33,1}}{5120}\)

\noindent\(C_{40,0000,0}^{20,0000,0,\text{NonLoc}}\longrightarrow \frac{7 C_{00,00}^{60,0}}{16384}+\frac{7 C_{00,00}^{60,1}}{8192}-\frac{7 \sqrt{3}
C_{00,20}^{60,0}}{16384}-\frac{7 \sqrt{3} C_{00,20}^{60,1}}{8192}+\frac{7 C_{11,00}^{51,0}}{16384}+\frac{7 C_{11,00}^{51,1}}{8192}+\frac{7 C_{20,00}^{40,0}}{16384}+\frac{7
C_{20,00}^{40,1}}{8192}-\frac{7 \sqrt{3} C_{20,20}^{40,0}}{16384}-\frac{7 \sqrt{3} C_{20,20}^{40,1}}{8192}+\frac{7 C_{22,00}^{42,0}}{8192 \sqrt{5}}+\frac{7
C_{22,00}^{42,1}}{4096 \sqrt{5}}-\frac{7 \sqrt{\frac{3}{5}} C_{22,20}^{42,0}}{8192}-\frac{7 \sqrt{\frac{3}{5}} C_{22,20}^{42,1}}{4096}+\frac{7 C_{31,00}^{31,0}}{16384}+\frac{7
C_{31,00}^{31,1}}{8192}-\frac{7 \sqrt{3} C_{31,20}^{31,0}}{16384}-\frac{7 \sqrt{3} C_{31,20}^{31,1}}{8192}+\frac{3 \sqrt{21} C_{33,00}^{33,0}}{40960}+\frac{3
\sqrt{21} C_{33,00}^{33,1}}{20480}-\frac{9 \sqrt{7} C_{33,20}^{33,0}}{40960}-\frac{9 \sqrt{7} C_{33,20}^{33,1}}{20480}\)

\noindent\(C_{40,2000,0}^{00,0000,0,\text{NonLoc}}\longrightarrow -\frac{7 C_{00,00}^{60,0}}{4096}-\frac{7 C_{00,00}^{60,1}}{2048}+\frac{7 \sqrt{3}
C_{00,20}^{60,0}}{4096}+\frac{7 \sqrt{3} C_{00,20}^{60,1}}{2048}-\frac{7 C_{11,00}^{51,0}}{12288}-\frac{7 C_{11,00}^{51,1}}{6144}+\frac{7 C_{11,20}^{31,0}}{4096
\sqrt{3}}+\frac{7 C_{11,20}^{31,1}}{2048 \sqrt{3}}-\frac{5 C_{20,00}^{40,0}}{12288}-\frac{5 C_{20,00}^{40,1}}{6144}+\frac{5 C_{20,20}^{40,0}}{4096
\sqrt{3}}+\frac{5 C_{20,20}^{40,1}}{2048 \sqrt{3}}+\frac{7 C_{22,00}^{42,0}}{6144 \sqrt{5}}+\frac{7 C_{22,00}^{42,1}}{3072 \sqrt{5}}-\frac{7 C_{22,20}^{42,0}}{2048
\sqrt{15}}-\frac{7 C_{22,20}^{42,1}}{1024 \sqrt{15}}+\frac{C_{31,00}^{31,0}}{12288}+\frac{C_{31,00}^{31,1}}{6144}-\frac{C_{31,20}^{31,0}}{4096 \sqrt{3}}-\frac{C_{31,20}^{31,1}}{2048
\sqrt{3}}+\frac{3 \sqrt{21} C_{33,00}^{33,0}}{10240}+\frac{3 \sqrt{21} C_{33,00}^{33,1}}{5120}-\frac{9 \sqrt{7} C_{33,20}^{33,0}}{10240}-\frac{9
\sqrt{7} C_{33,20}^{33,1}}{5120}\)

\noindent\(C_{60,0000,0}^{00,0000,0,\text{NonLoc}}\longrightarrow \frac{C_{00,00}^{60,0}}{16384}+\frac{C_{00,00}^{60,1}}{8192}-\frac{\sqrt{3} C_{00,20}^{60,0}}{16384}-\frac{\sqrt{3}
C_{00,20}^{60,1}}{8192}+\frac{C_{11,00}^{51,0}}{16384}+\frac{C_{11,00}^{51,1}}{8192}-\frac{\sqrt{3} C_{11,20}^{31,0}}{16384}-\frac{\sqrt{3} C_{11,20}^{31,1}}{8192}+\frac{C_{20,00}^{40,0}}{16384}+\frac{C_{20,00}^{40,1}}{8192}-\frac{\sqrt{3}
C_{20,20}^{40,0}}{16384}-\frac{\sqrt{3} C_{20,20}^{40,1}}{8192}+\frac{C_{22,00}^{42,0}}{8192 \sqrt{5}}+\frac{C_{22,00}^{42,1}}{4096 \sqrt{5}}-\frac{\sqrt{\frac{3}{5}}
C_{22,20}^{42,0}}{8192}-\frac{\sqrt{\frac{3}{5}} C_{22,20}^{42,1}}{4096}+\frac{C_{31,00}^{31,0}}{16384}+\frac{C_{31,00}^{31,1}}{8192}-\frac{\sqrt{3}
C_{31,20}^{31,0}}{16384}-\frac{\sqrt{3} C_{31,20}^{31,1}}{8192}+\frac{3 \sqrt{\frac{3}{7}} C_{33,00}^{33,0}}{40960}+\frac{3 \sqrt{\frac{3}{7}} C_{33,00}^{33,1}}{20480}-\frac{9
C_{33,20}^{33,0}}{40960 \sqrt{7}}-\frac{9 C_{33,20}^{33,1}}{20480 \sqrt{7}}\)

\end{document}
